# Supplementary material for: Structured Domain Adaptation with Online Relation Regularization for Unsupervised Person Re-ID
Source: arXiv:2003.06650 source file (2022-05-05)
Supplement: Supplementary file 1 [file SDA_Appendix.pdf]

# Structured Domain Adaptation with Online Relation Regularization for Unsupervised Person Re-ID

## Supplementary Material

Anonymous Author(s)

Affiliation

Address

email

### 1 A Comparison with Domain Translation-based UDA Methods

#### 2 A.1 Domain Translated Examples

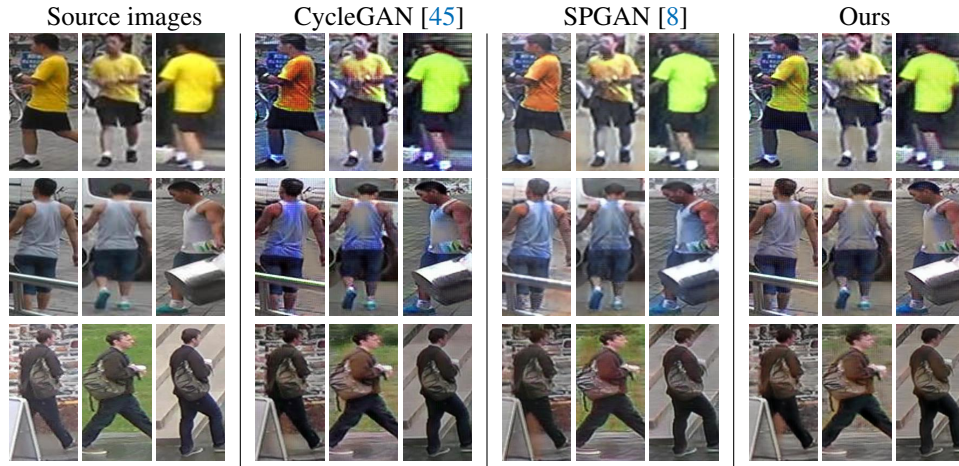

**Figure 3.** Domain-translated examples of CycleGAN [45], SPGAN [8] and our method. SPGAN adopts ID-based regularizations (*i.e.*, contrastive loss), showing inferior generation results than our method. ID-based regularizations are too weak to preserve inter-sample relations during translation. For instance, the man in the first row appears to be in different colors (*e.g.*, orange, yellow and green) within a tuple after translation by CycleGAN and SPGAN. Other translation-based methods [36, 9, 3] did not provide trained models or translated images, thus not be illustrated here. However, we have carefully discussed and compared them with their ID-based regularizations in the ablation studies mentioned above. Best viewed in color.

#### 3 A.2 Performance of Target-domain Encoder w/o Pseudo Labels

**Table 5.** Comparison with domain translation-based UDA methods using target-domain encoder **without** pseudo labels. The performances (%) are reported on DukeMTMC-reID [29] and Market-1501 [40] datasets.

| Methods w/o Pseudo Labels | DukeMTMC-reID→Market-1501 |             |             |             | Market-1501→DukeMTMC-reID |             |             |             |
|---------------------------|---------------------------|-------------|-------------|-------------|---------------------------|-------------|-------------|-------------|
|                           | mAP                       | top-1       | top-5       | top-10      | mAP                       | top-1       | top-5       | top-10      |
| PTGAN [36] (CVPR'18)      | -                         | 38.6        | -           | -           | -                         | 27.4        | -           | -           |
| SPGAN [8] (CVPR'18)       | 22.8                      | 51.5        | 70.1        | 76.8        | 22.3                      | 41.1        | 56.6        | 63.0        |
| M2M-GAN [22] (AAAI'19)    | 26.8                      | 57.5        | -           | -           | 26.1                      | 49.6        | -           | -           |
| CR-GAN [3] (ICCV'19)      | 29.6                      | 59.6        | -           | -           | 30.0                      | 52.2        | -           | -           |
| Our SDA w/o pseudo labels | <b>35.0</b>               | <b>64.5</b> | <b>79.5</b> | <b>84.6</b> | <b>34.3</b>               | <b>53.1</b> | <b>67.1</b> | <b>72.4</b> |

4 In the original paper’s Table 4, we evaluated our proposed online relation-consistency regularization  
5 by replacing  $\mathcal{L}_{rc}$  with previous ID-based regularizations [8, 9, 3] in our final framework.

6 To further verify the effectiveness of our structured domain translation for domain adaptation, we  
7 evaluate our framework using a target-domain encoder **without** pseudo labels, which is a common  
8 strategy in previous translation-based methods [36, 8, 22, 3], *i.e.*, the target-domain encoder is trained  
9 with only source-to-target translated images and their source-domain identities. As shown in Table 5,  
10 our method stably achieves state-of-the-art performances on both Duke→Market and Market→Duke  
11 adaptation tasks without generating pseudo labels in the target domain.

### 12 A.3 Performance w/o Joint Training of SDT and Target-domain Encoder

**Table 6.** Comparison with domain translation-based UDA methods with pseudo labels (via  $k$ -means clustering) but **without** jointly training the domain-translation network and target-domain encoder. The performances (%) are reported on DukeMTMC-reID [29] and Market-1501 [40] datasets.

| Methods w/o Joint Training                    | DukeMTMC-reID→Market-1501 |             |             |             | Market-1501→DukeMTMC-reID |             |             |             |
|-----------------------------------------------|---------------------------|-------------|-------------|-------------|---------------------------|-------------|-------------|-------------|
|                                               | mAP                       | top-1       | top-5       | top-10      | mAP                       | top-1       | top-5       | top-10      |
| Baseline (target-domain data + pseudo labels) | 59.0                      | 80.7        | 90.5        | 93.4        | 50.1                      | 68.2        | 79.2        | 82.7        |
| Base. + source-to-target data by CycleGAN     | 56.0                      | 79.6        | 90.6        | 93.9        | 51.2                      | 69.5        | 80.4        | 83.5        |
| Base. + source-to-target data by SPGAN [8]    | 53.6                      | 78.3        | 89.6        | 92.8        | 48.9                      | 64.3        | 78.4        | 83.6        |
| Base. + source-to-target data by our SDT      | <b>61.3</b>               | <b>83.3</b> | <b>91.8</b> | <b>94.9</b> | <b>54.3</b>               | <b>71.6</b> | <b>82.0</b> | <b>85.6</b> |

13 The domain-translation network and target-domain encoder in our framework promote each other via  
14 joint training. However, a simpler training scheme would be to first train a source-to-target translation  
15 network with the proposed regularization and translate all source-domain images to the target domain.  
16 A pseudo-label-based target-domain encoder is then trained with such fixed source-to-target translated  
17 images and target-domain images.

18 We evaluate both our framework and existing translation-based methods [45, 8] when adopting  
19 such separate training strategy and  $k$ -means clustering for pseudo label generation. The results in  
20 Table 6 show that the informative training samples generated by our proposed structured domain-  
21 translation (SDT) network could effectively improve the already strong baseline even without our  
22 joint training scheme, while the source-to-target images generated by CycleGAN and SPGAN might  
23 even worsen the performance because their generated images might not well follow the distributions  
24 of target-domain data and maintain their original inter-sample relations.
